# Supplementary material for: PromptST: Prompt-Enhanced Spatio-Temporal Multi-Attribute Prediction
Source: arXiv:2309.09500 source file (2023-09-18)
Supplement: Supplementary file 1 [file 8_Appendix.tex]

\section{Technical Appendix}

\subsection{Framework Illustration}
\label{subsec:alg}
We present the pipeline of spatio-temporal transformer in Algorithm \ref{alg:algorithm1}.
Basically, we feed the spatio-temporal transformer with feature matrix of all attributes in parallel (line 1). 
For spatio-temporal feature matrix of each attribute $\boldsymbol{X}_c$, we capture the temporal and spatial dependency, respectively.
In temporal encoder, we first map the feature into embedding space (line 3), and add positional embedding (line 4).
Then, we conduct $l_t$ layers of multi-head attention and feed-forward layer sequentially (lines 5-7).
At last, we take the last timestep of the feature matrix as the temporal representation (line 8).
In spatial encoder, we add spatially positional information first (line 10). 
Similarly, we process the feature matrix with $l_s$ layers of multi-head attention and feed-forward layer sequentially (lines 11 to 14).
Then, we map the learned spatial representation with an MLP-based head to spatio-temporal attribute of future timesteps (lines 15 and 16).
Finally, the spatio-temporal transformer concatenates and returns the $C$ spatio-temporal attributes (line 18).

\begin{algorithm}[htbp]
	\caption{\label{alg:algorithm1} 
    The pipeline of spatio-temporal transformer $f_{\boldsymbol{W}}(\boldsymbol{\mathcal{X}})$. 
	% Optimizing pipeline of \name.
	}
	\raggedright
	{\bf Input}:  Historical spatio-temporal attributes $\boldsymbol{\mathcal{X}}$.
 \\
	{\bf Output}: Predicted spatio-temporal attributes $\boldsymbol{\mathcal{\hat{Y}}}$.\\
    % \textbf{Stage 1. Pretrain the spatio-temporal transformer.}\\
	\begin{algorithmic} [1]
        % \State \textbf{Stage I. Pretrain the spatio-temporal transformer.}
        \For{$\boldsymbol{X}_c$ in $\boldsymbol{\mathcal{X}}=[\boldsymbol{X}_1, \ldots, \boldsymbol{X}_c, \ldots, \boldsymbol{X}_C]$}
        \State // Temporal encoder. %\Comment{step1}\\
        \State $\boldsymbol{\mathcal{Z}} = \sigma(\boldsymbol{W}_m {\rm Trans}(\boldsymbol{{X}}_c)+\boldsymbol{b}_m)$ \Comment{Eq. \eqref{Equ:bottom}}
        % Transform $\boldsymbol{X}_c$ into embedding space and attain $\boldsymbol{\mathcal{Z}}$ by Eq. \eqref{Equ:bottom}.\\
	    \State $\boldsymbol{\mathcal{Z}}_{temp}^{(0)} = \boldsymbol{\mathcal{Z}}+\boldsymbol{p}_{temp}$ \Comment{Eq. \eqref{Equ:temporal_position}}
     % Add temporal positional embedding to $\boldsymbol{\mathcal{Z}}$ as Eq. \eqref{Equ:temporal_position}.\\
    	\For{$l$ in $1, \ldots, l_t$}
        \State
        $\boldsymbol{\mathcal{Z}}_{temp}^{(l)} = F(M(\boldsymbol{\mathcal{Z}}_{temp}^{(l-1)}))$ \Comment{Eq. \eqref{Equ:TempEncoder}}
        % $\boldsymbol{\mathcal{Z}}_{temp}^{(l-1)} = LayerNorm(\boldsymbol{\mathcal{Z}}_{temp}^{(l-1)}, MHAtt(\boldsymbol{\mathcal{Z}}_{temp}^{(l-1)},\boldsymbol{\mathcal{Z}}_{temp}^{(l-1)},\boldsymbol{\mathcal{Z}}_{temp}^{(l-1)}))$\\
        % \State $\boldsymbol{\mathcal{Z}}_{temp}^{(l-1)} = LayerNorm(\boldsymbol{\mathcal{Z}}_{temp}^{(l-1)}+FeedFwd(\boldsymbol{\mathcal{Z}}_{temp}^{(l-1)}))$\\
        % \State $\boldsymbol{\mathcal{Z}}_{temp}^{(l)} = \boldsymbol{\mathcal{Z}}_{temp}^{(l-1)}$\\
        \EndFor
        \State $\boldsymbol{\mathcal{Z}}_{temp} = \boldsymbol{\mathcal{Z}}_{temp}^{(l_t)}\Big|_{t=T}$ \Comment{Eq. \eqref{Equ:TempRepresentation}}
        \State // Spatial encoder. 
        \State $\boldsymbol{\mathcal{Z}}_{spa}^{(0)} = \boldsymbol{\mathcal{Z}}_{temp}+\boldsymbol{p}_{spa}
        %+{\rm PE}(\boldsymbol{\mathcal{Z}}_{temp}) 
        $ \Comment{Eq. \eqref{Equ:spatial_position}}
        \For{$l$ in $1,\ldots,l_s$}
        \State 
        $\boldsymbol{\mathcal{Z}}_{spa}^{(l)} = F(M(\boldsymbol{\mathcal{Z}}_{spa}^{(l-1)}))$ \Comment{Eq. \eqref{Equ:SpaEncoder}}
        % $\boldsymbol{\mathcal{Z}}_{spa}^{(l-1)} = LayerNorm(\boldsymbol{\mathcal{Z}}_{spa}^{(l-1)}, MHAtt(\boldsymbol{\mathcal{Z}}_{spa}^{(l-1)},\boldsymbol{\mathcal{Z}}_{spa}^{(l-1)},\boldsymbol{\mathcal{Z}}_{spa}^{(l-1)}))$\\
        % \State $\boldsymbol{\mathcal{Z}}_{spa}^{(l-1)} = LayerNorm(\boldsymbol{\mathcal{Z}}_{spa}^{(l-1)}+FeedFwd(\boldsymbol{\mathcal{Z}}_{spa}^{(l-1)}))$\\
        % \State $\boldsymbol{\mathcal{Z}}_{spa}^{(l)} = \boldsymbol{\mathcal{Z}}_{spa}^{(l-1)}$\\
	    \EndFor
        \State $\boldsymbol{\mathcal{Z}}_{spa} = \boldsymbol{\mathcal{Z}}_{spa}^{(l_t)}$ \Comment{Eq. \eqref{Equ:SpaRepresentation}}
        \State // Head.
        \State $\boldsymbol{\hat{Y}}_c = \sigma(\boldsymbol{W}_h\boldsymbol{\mathcal{Z}}_{spa}+\boldsymbol{b}_h)$ \Comment{Eq. \eqref{Equ:head}}
        \EndFor
        \State $\boldsymbol{\mathcal{\hat{Y}}}=[\boldsymbol{\hat{Y}}_1, \ldots, \boldsymbol{\hat{Y}}_c, \ldots, \boldsymbol{\hat{Y}}_C]$
    	\raggedright
	    \State
	    {\bf Return}: $\boldsymbol{\mathcal{\hat{Y}}}$
	\end{algorithmic}
\end{algorithm}

Based on spatio-temporal transformer defined in Section \ref{subsec:sttransformer}, the pretrain and prompt tuning procedure are shown as in Algorithm \ref{alg:algorithm2}.
% If t
Tuning with \stpmt, we replace Eq. \eqref{Equ:TempEncoder} in $f_{\boldsymbol{W}}(\boldsymbol{\mathcal{X}})$ with Eq. \eqref{Equ:stpmtTempEncoder} and get $f_{\boldsymbol{W}}^{st}(\boldsymbol{\mathcal{X}})$ (line 10).
% If tuning with \apmt, we replace Eq. \eqref{Equ:TempEncoder}  and Eq. \eqref{Equ:SpaEncoder} in $f_{\boldsymbol{W}}(\boldsymbol{\mathcal{X}})$ with Eq. \eqref{Equ:apmtTempEncoder} and Eq. \eqref{Equ:apmtSpaEncoder}, respectively, and get $f_{\boldsymbol{W}}^{ti}(\boldsymbol{\mathcal{X}})$ (line 13 to 15).
By only optimizing the small scale of parameters $\boldsymbol{\gamma},\boldsymbol{\omega}$ (lines 11 and 12), \name can well address the spaio-temporal characteristic of specific attribute.
% Prompt tuning with \stpmt replace Eq. \eqref{Equ:TempEncoder} with Eq. \eqref{Equ:stpmtTempEncoder}. 
% Prompt tuning with \apmt replace Eq. \eqref{Equ:TempEncoder} with Eq. \eqref{Equ:apmtTempEncoder}, and Eq. \eqref{Equ:SpaEncoder} with Eq. \eqref{Equ:apmtSpaEncoder}.
\begin{figure}[!t]
\centering
	%	\hspace*{-7mm}1.049
	\includegraphics[width=0.9\linewidth]{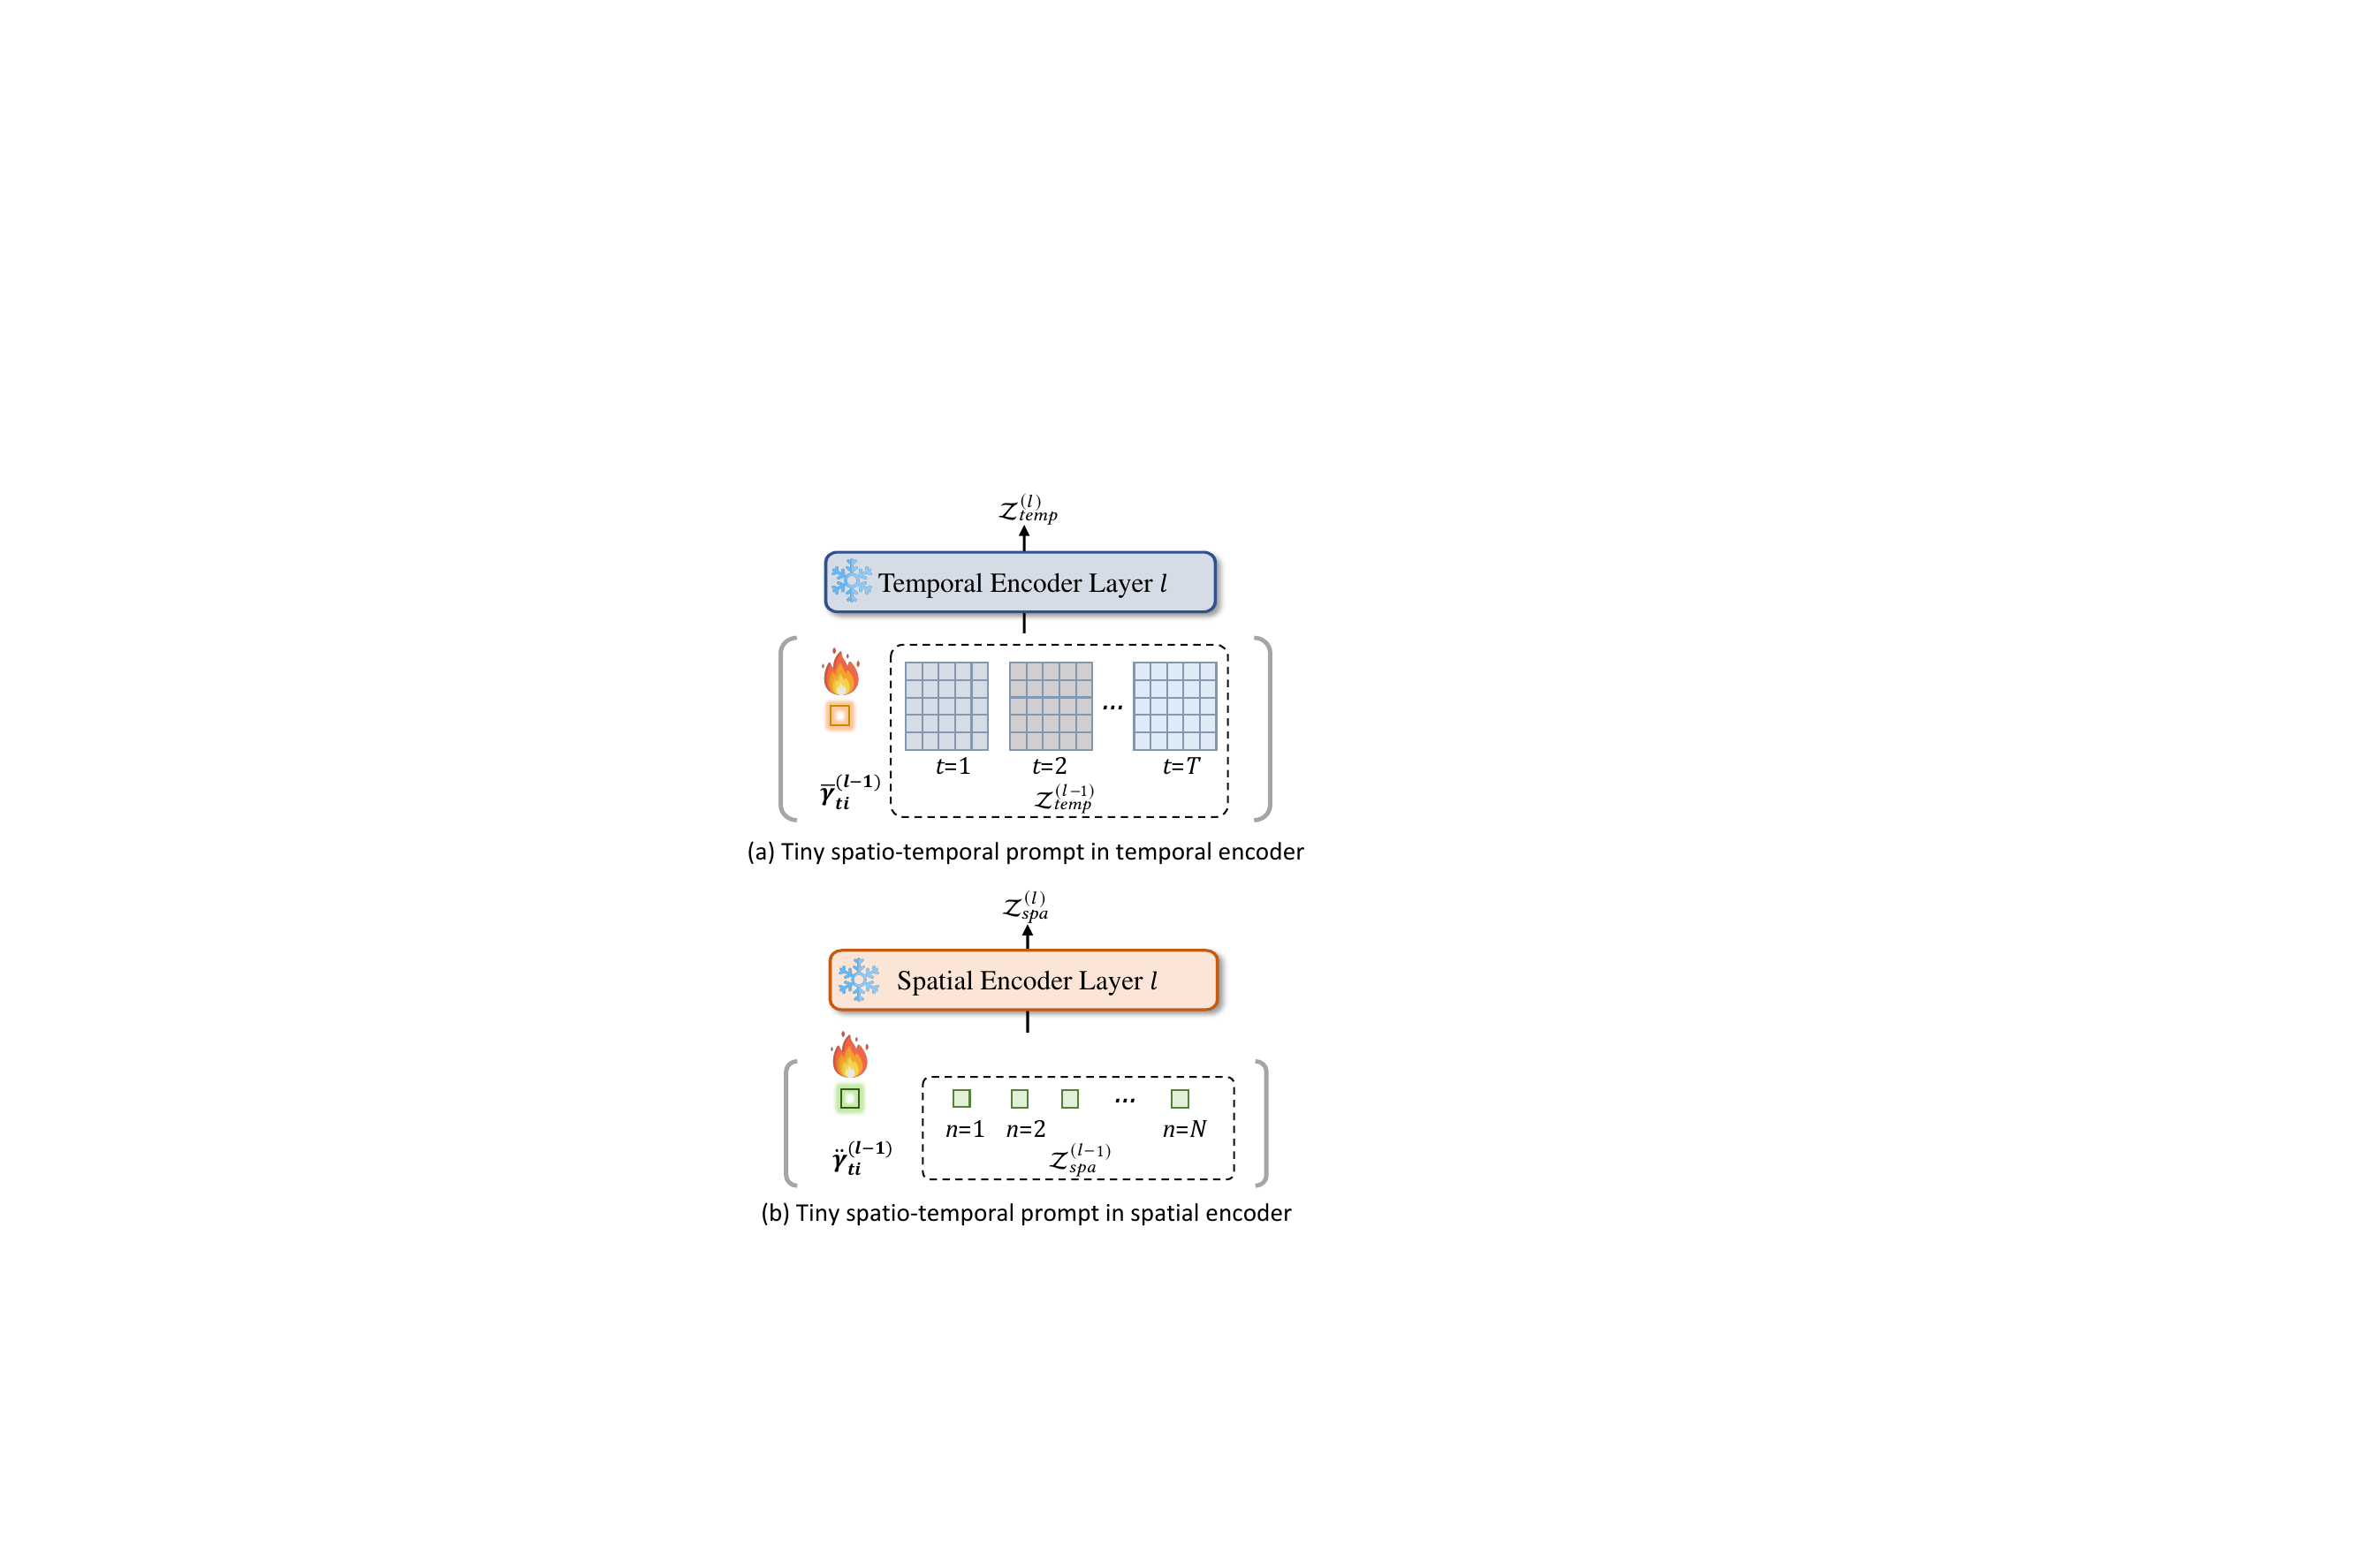}
	\caption{Prompt tuning with \apmt, the luminous grids represent the prompt tokens. \name keeps the main body frozen and updates the prompt tokens and head. 
    Tiny spatio-temporal prompt inserts prompt tokens to feature {(a)} sequence of temporal encoder, and (b) sequence of spatial encoder.
 }
	\label{fig:promptti}
	\vspace*{-3mm}
\end{figure}
\begin{algorithm}[htbp]
	\caption{\label{alg:algorithm2}  
	Optimizing pipeline of \name.
	}
	\raggedright
	{\bf Input}:  Historical spatio-temporal attributes $\boldsymbol{\mathcal{X}}$, and future spatio-temporal attributes $\boldsymbol{\mathcal{{Y}}}$.
 \\
	{\bf Output}: Well-trained spatio-temporal transformer $f_{\boldsymbol{\gamma},\boldsymbol{\omega}}(\boldsymbol{\mathcal{X}})$.\\
	\begin{algorithmic} [1]
    \State \textbf{Phase I.} Pretrain the spatio-temporal transformer $f_{\boldsymbol{\theta},\boldsymbol{\omega}}(\boldsymbol{\mathcal{X}})$.
        \While{not converge}
        \State $\boldsymbol{\mathcal{\hat{Y}}} = f_{\boldsymbol{\theta},\boldsymbol{\omega}}(\boldsymbol{\mathcal{X}})$
        \State $\mathcal{L} = 
        {\rm RMSE}( \boldsymbol{\mathcal{\hat{Y}}},\boldsymbol{\mathcal{Y}})+
        {\rm MAE}(\boldsymbol{\mathcal{\hat{Y}}},\boldsymbol{\mathcal{Y}})$
        \State Update $\boldsymbol{\theta}$ and $\boldsymbol{\omega}$ by gradient descent by $\partial_{\boldsymbol{\theta}}\mathcal{L}$ and $\partial_{\boldsymbol{\omega}}\mathcal{L}$.
        \EndWhile
	% \end{algorithmic}
    \State \textbf{Phase II.} Prompt tune the spatio-temporal transformer $f_{\boldsymbol{\gamma},\boldsymbol{\omega}}(\boldsymbol{\mathcal{X}})$.
	% \begin{algorithmic} [1]
        \State For spatio-temporal transformer $f_{\boldsymbol{\theta},\boldsymbol{\omega}}(\boldsymbol{\mathcal{X}})$ parameterized with $\boldsymbol{\theta}$ and $\boldsymbol{\omega}$, fix parameters $\boldsymbol{\theta}$, and initialize $\boldsymbol{\omega}$.
        \While{not converge}
        % \If{$\boldsymbol{\gamma}=\boldsymbol{\gamma}_{st}$}
        % \State // Tune with \stpmt.
        \State $\boldsymbol{\mathcal{\hat{Y}}} = f_{\boldsymbol{\gamma},\boldsymbol{\omega}}^{st} (\boldsymbol{\mathcal{X}})$
        % \Else
        % \State // Tune with \apmt.
        % \State $\boldsymbol{\mathcal{\hat{Y}}} = f_{\boldsymbol{\gamma},\boldsymbol{\omega}}^{ti} (\boldsymbol{\mathcal{X}})$        
        % \EndIf
        \State$\mathcal{L} = 
        {\rm RMSE}( \boldsymbol{\mathcal{\hat{Y}}},\boldsymbol{\mathcal{Y}})+
        {\rm MAE}(\boldsymbol{\mathcal{\hat{Y}}},\boldsymbol{\mathcal{Y}})$
        \State Update $\boldsymbol{\gamma}$ and $\boldsymbol{\omega}$ by gradient descent by $\partial_{\boldsymbol{\gamma}}\mathcal{L}$ and $\partial_{\boldsymbol{\omega}}\mathcal{L}$.

        \EndWhile
	    \State
	    {\bf Return}: $f_{\boldsymbol{\gamma},\boldsymbol{\omega}}(\boldsymbol{\mathcal{X}})$ with the optimal $\boldsymbol{\gamma}, \boldsymbol{\omega}$.
	\end{algorithmic}
 % \vspace{-5mm}
\end{algorithm}

\subsection{Dataset and Baseline Setups}
\label{subsec:baselines}
In this subsection, we briefly introduce the datasets we used, then we present the advancing baselines in this paper and detail the experimental setups.

\begin{table}[h]
\begin{center}
\vspace{-1mm}
	\caption{Statistics of the datasets.
}
	\vspace{-3.1mm}
	\label{table:datainfo}
	\scalebox{0.95}{
	\begin{tabular}{@{}|c|c|c|@{}}
		\toprule[1pt]
		\textbf{Dataset} & \multicolumn{1}{c|}{\textbf{Complaint}} & \textbf{NYC Taxi} \\ \midrule
\# attributes & 19 & 4\\
\midrule
\# trajectories & 2.27 M & 14.09 M\\%165.11 M
\midrule
time span & 1/1/2013$\sim$31/12/2014 & 1/1/2014$\sim$31/3/2014 \\ % 1/1/2014$\sim$31/12/2014
\midrule
grid shape & (8, 8) & (10, 20)\\
\midrule
time interval & 3 h & 20 min \\ %1 h
		\bottomrule[1pt]
	\end{tabular}}
	\vspace{-2mm}
\end{center}
\end{table}

\begin{itemize}[leftmargin=*]
    \item \textbf{ARIMA \cite{arima}}: Autoregressive integrated moving average model is a representative statistic method for time series prediction.
    
    \item \textbf{Conv-GCN \cite{convgcn}}: Conv-GCN combines a graph neural network with a three-dimensional convolution neural network to address the spatial and temporal relationship.
    
    \item \textbf{HGCN \cite{hgcn}}: Hierarchical graph convolutional network forecast spatio-temporal attributes by operating on both the micro and macro traffic graphs.
    
    \item \textbf{ASTGCN \cite{astgcn}}: It proposes an attention-based graph convolutional network and addresses multiple temporal properties to solve spatio-temporal prediction.
    
    \item \textbf{CCRNN \cite{ccrnn}}: The coupled layer-wise convolutional recurrent neural network incorporates adaptive adjacency matrices for each graph convolution network layer.
    
    \item \textbf{MTGNN \cite{mtgnn}}: It incorporates a mix-hop propagation layer in graph neural networks to address multi-variate time series prediction.
    
    \item \textbf{GTS \cite{gts}}: GTS is an efficient solution for graph structure learning as a probabilistic graph model.
\end{itemize}

To achieve a comprehensive comparison, we also modify some advancing baselines in spatio-temporal multivariate prediction:
\textbf{ASTGCN-Full}, \textbf{CCRNN-Full}, and \textbf{MTGNN-Full}.
Due to the situation that their original goals are to predict single spatio-temporal attributes, we upgrade the input dimension from 1 to 19 on Complaint, and to 4 on NYC Taxi.

In this paper, we propose an effective spatio-temporal transformer and train it in a parameter-sharing way.
To verify the \name from multiple viewpoints, we optimize the spatio-temporal transformer in several training strategies: 

\begin{itemize}[leftmargin=*]
    \item \textbf{Single-Train}: We iteratively train the spatio-temporal transformer from scratch on all the attributes. For example, we train spatio-temporal transformer 19 times on Complaint, and each time it feeds on one attribute. 
    
    \item \textbf{Full-Train}: We input all attributes into spatio-temporal transformer together and train in a parameter-sharing way.
    
    \item \textbf{Fine-Tune}: We load the pretrained/full-trained backbone and tune all model parameters on each attribute, respectively.
\end{itemize}

\begin{table}[htbp]
	\caption{All the 19 types of complaints in Complaint dataset.}
\label{table:complaint}
\begin{tabular}{l|c}\toprule
\textbf{Complaint Type}     & \textbf{Amount} \\\midrule
Noise - Commercial &  63,745      \\\midrule
PAINT/PLASTER      &  64,381      \\\midrule
ELECTRIC &  64,923 \\\midrule
Dirty Conditions  &  63,931      \\\midrule
 Sewer                  &  66,518     \\\midrule
  Traffic Signal Condition                 &  51,522     \\\midrule
 PAINT - PLASTER                  & 88,838      \\\midrule
 Noise                  &  90,021     \\\midrule
 General Construction/Plumbing                  & 55,175      \\\midrule
  Illegal Parking                 &  106,857     \\\midrule
  Water System                 &  107,979     \\\midrule
   GENERAL CONSTRUCTION                & 126,360      \\\midrule
  HEAT/HOT WATER                 &   132,756    \\\midrule
  Blocked Driveway                &   136,488    \\\midrule
   PLUMBING                &    148,409   \\\midrule
  Street Light Condition                 &  105,018     \\\midrule
  Street Condition                 &  164,532     \\\midrule
  HEATING                 &   289,940    \\\midrule
   Noise - Residential                &  343,588     \\
		\bottomrule[1pt]
\end{tabular}
\end{table}

\subsection{Implementation Details}
\label{subsec:implementation}
\subsubsection{\zzj{
Notation Definition
}}
\zzj{
[Notation Table]
}

\subsubsection{Full List of Complaint Type}
We pick up the complaint records in 2013 and 2014, and get 19 attributes with the largest amounts. The full 19 complaint types and corresponding amounts are shown in Table \ref{table:complaint}.

\subsubsection{Setup of \name}
Our model and all the baselines are implemented with PyTorch. 
We evaluate the methods on a Linux server with one NVIDIA 2080ti GPU.
For \name, we incorporate a temporal encoder with 2 layers, and a spatial encoder with 2 layers. The head is with a shape of 32$\times 12$. 
In pretrain stage, we set the learning rate as 0.003, batch size as 32.
For fine-tune stage, we set the learning rate as 0.001, batch size as 32.
For prompt-tune stage, we set the learning rate as 0.001, batch size as 32. We insert 2 \stpmt to each temporal encoder layer.
The learning parameters of the backbone are initialized with a uniform distribution. The prompt tokens are initialized with xavier initialization.

\subsubsection{Set of Baselines}
To foster a fair comparison, we tune the hyper-parameters of baseline models. We utilize the open-source platform LibCity\footnote{\url{https://libcity.ai/\#/}} for baseline implementation.
The detailed hyper-parameters are listed as Table \ref{table:setupbaseline}.

\subsection{\apmthead}
\label{subsec:tiny}
Based on spatio-temporal transformer defined in Section \ref{subsec:sttransformer}, and the pretrain and prompt tuning procedure in Algorithm \ref{alg:algorithm2}, we describe the pipeline of prompt tuning with \apmt. 
After pretrainin the backbone spatio-temporal transformer, 
to tune with \apmt, we replace Eq. \eqref{Equ:TempEncoder}  and Eq. \eqref{Equ:SpaEncoder} in $f_{\boldsymbol{W}}(\boldsymbol{\mathcal{X}})$ with Eq. \eqref{Equ:apmtTempEncoder} and Eq. \eqref{Equ:apmtSpaEncoder}, respectively, and get $f_{\boldsymbol{W}}^{ti}(\boldsymbol{\mathcal{X}})$.

\begin{table}[h]
\begin{center}
	\caption{Baselines hyper-parameters setup.
}
	\vspace{-3.1mm}
	\label{table:setupbaseline}
	\scalebox{0.85}{
	\begin{tabular}{@{}|c|c|c|c|c|@{}}
		\toprule[1pt]
% 		\textbf{hyper-parameter}
        Methods & setting & batch size & learning rate & embedding size \\
% 		Multi-Tasks & In \& Out & OD \& Duration & Flow \& Speed\\ 
\midrule
\multirow{1}{*}{Conv-GCN}
 & Single-Train & 64 & 0.003 & 64 \\%& 1e-6\\
\midrule
\multirow{1}{*}{HGCN}
 & Single-Train & 64 & 0.003 & 64 \\%& 1e-6\\
\midrule
\multirow{1}{*}{GTS}
 & Single-Train & 64 & 0.003 & 64 \\%& 1e-6\\
\midrule
\multirow{2}{*}{ASTGCN}
 & Single-Train & 64 & 0.003 & 64 \\%& 1e-6\\
 & Full-Train & 32 & 0.003 & 64 \\%& 1e-6\\
\midrule
\multirow{2}{*}{CCRNN}
 & Single-Train & 64 & 0.001 & 64\\ %& 1e-6\\
 & Full-Train & 32 & 0.001 & 64 \\%& 1e-6\\
\midrule
\multirow{2}{*}{MTGNN}
 & Single-Train & 64 & 0.001 & 64\\ %& 1e-6\\
 & Full-Train & 32 & 0.001 & 64 \\%& 1e-6\\
%& 1e-6\\
		\bottomrule[1pt]
	\end{tabular}}
	\vspace{-5.1mm}
\end{center}
\end{table}
